# Supplementary material for: The Imperative of Conversation Analysis in the Era of LLMs: A Survey of Tasks, Techniques, and Trends
Source: arXiv:2409.14195 source file (2024-09-21)
Supplement: Supplementary file 1 [file appendix.tex]

\clearpage
\appendix

\begin{equation}
\begin{aligned}
    \max f_{\Theta}(\mathcal{D}) \rightarrow \mathcal{G} \\

\label{eq-com}
\end{aligned}
\end{equation}
